# Supplementary material for: Multi-Objective Path-Based D* Lite
Source: arXiv:2108.00710 source file (2022-01-21)
Supplement: Supplementary file 1 [file appendix.tex]

\graphicspath{{figures/}}

\subsection{Motivating Example for Multi-objective Path Planning}

\begin{figure*}[htbp]
	\centering
	\vspace{-0mm}
	\includegraphics[width=0.8\linewidth,height=6.4cm]{mospp_example.png}
	\vspace{-2mm}
	\caption{A motivating example for multi-objective path planning. The task is to plan path connecting the start (green cell) and the destination (blue cell) while optimizing both path risk and length. There are three Pareto-optimal solutions as shown in (c) and (e). Using a scalarization-based aproach as shown in (f), however, can never find the orange solution path. Plot (d) helps illustrate the reason behind and more details can be found in the text.}
	%	\vspace{-4mm}
	\label{fig:mospp_example}
	\vspace{-3mm}
\end{figure*}

One simple approach that solves multi-objective planning is to scalarize multiple objectives into a single one via linear weighting and then resort to existing single-objective planner such as A*, D* Lite, etc, to solve the scalarized problem.
We provide an example that illustrate the limitation of such scalarization approach.
As shown in Fig.~\ref{fig:mospp_example}, the task is to plan paths for a robot in some uneven terrain, which is represented as a four-connected occupancy grid (Fig.~\ref{fig:mospp_example}(b)), from the given start (cell with green boundary) to destination (cell with blue boundary).
The risk score of a cell is equal to the number of obstacles in the proximity (Fig.~\ref{fig:mospp_example}(a)), which describes the potential collision risk with the obstacle.
This task minimizes both path length (number of actions of the robot) and accumulated risk along the path.
With an exact multi-objective planner (such as NAMOA*, MOPBD*), the Pareto-optimal set of solutions can be computed, which is shown in Fig.~\ref{fig:mospp_example}(c). The cost vectors of these solutions are reported in Fig.~\ref{fig:mospp_example}(e) and the corresponding Pareto-optimal front is visualized in Fig.~\ref{fig:mospp_example}(d).
With this Pareto-optimal front in hand, the decision maker (human or another decision making software) can choose the best solution to be executed based on domain knowledge.
In this example, let's assume that the decision maker prefers the orange solution in Fig.~\ref{fig:mospp_example}(c) due to its balance between risk and length.

Now, let's consider using a scalarization-based approach to solve the problem. The cost vector associated with each edge $\vec{c}(e)$ can be readily scalarized via linear weighting:
\begin{eqnarray}\label{eqn:scalarization}
	c'(e) = w\cdot c_1(e) + (1-w)\cdot c_2(e)
\end{eqnarray}
, where $c'$ denote the scalarized cost, $c_1$, $c_2$ denote path length (which is always one for each edge) and risk score respectively and $w \in [0,1]$ denote weight factor (i.e. preference) between path length and risk.
By varying $w$ between zero and one, the MO-SPP is transformed into a (single-objective) SPP, which can be then solved via existing path planners (such as A*, D* Lite).
Fig.~\ref{fig:mospp_example}(f) reports the scalarized cost value of all three Pareto-optimal paths under different $w$ (with a step size of $0.1$ betwen $[0,1]$) and the optimal solution computed by single-objective planner is marked in bold.
It turns out that no matter which $w$ we choose, the scalarization method never find the orange solution in Fig.~\ref{fig:mospp_example}(c), as the scalarized cost of the orange solution is never the minimum.

We provide a brief analysis for this example to get an intuitive understanding of the reason behind.
As the scalarized cost of a path $g'(\pi)$ is the sum of costs of edges present in the path $\pi$, with equation (\ref{eqn:scalarization}), we get $g'(\pi) = w\cdot g_1(\pi) + (1-w)\cdot g_2(\pi)$, where $g_1$ and $g_2$ are path length and path risk respectively.
When $w\neq 1$, this can be rewritten into the form of a line: $g_2(\pi) = \frac{-w}{1-w}\cdot g_1(\pi) + \frac{1}{1-w} g'(\pi)$, where $\frac{-w}{1-w}$ is the slope of the line while $\frac{1}{1-w} g'(\pi)$ is the intercept.
Given a $w$, the slope of the line is fixed and an optimal solution $\pi_*$ of the scalarized SPP (of that $w$) must locate on the line with the minimum intercept.
As shown in Fig.~\ref{fig:mospp_example}(d), for this example, the optimal solution returned by the scalarization method can never go through the orange dot, which is on the dashed black line, since the solid black line has the same slope as the dashed black line and achieves less intercept.
We refer the reader to \cite{emmerich2018tutorial} for more discussion on scalaraization method.
